# Supplementary material for: Enhanced search for neutral current $\Delta$ radiative single-photon production in MicroBooNE
Source: arXiv:2502.05750 ancillary file (2025-11-17)
Supplement: Supplementary file 1 [file enhanced_NC_Delta_supplement.pdf]

# Supplemental Material

## Appendix A: Constraining Sidebands

Figure 6 shows the sideband observations used in all constrained predictions. The NC  $\pi^0$  selections are binned from 0-1500 MeV of reconstructed energy transfer (reconstructed energy not carried away by the exiting neutrino), with an overflow bin. The  $\nu_\mu$ CC selections are binned from 0-1500 MeV of reconstructed neutrino energy, with an overflow bin. The  $\chi^2/\text{ndf}$  for all four channels is 46.89/64, representing good agreement within uncertainties.

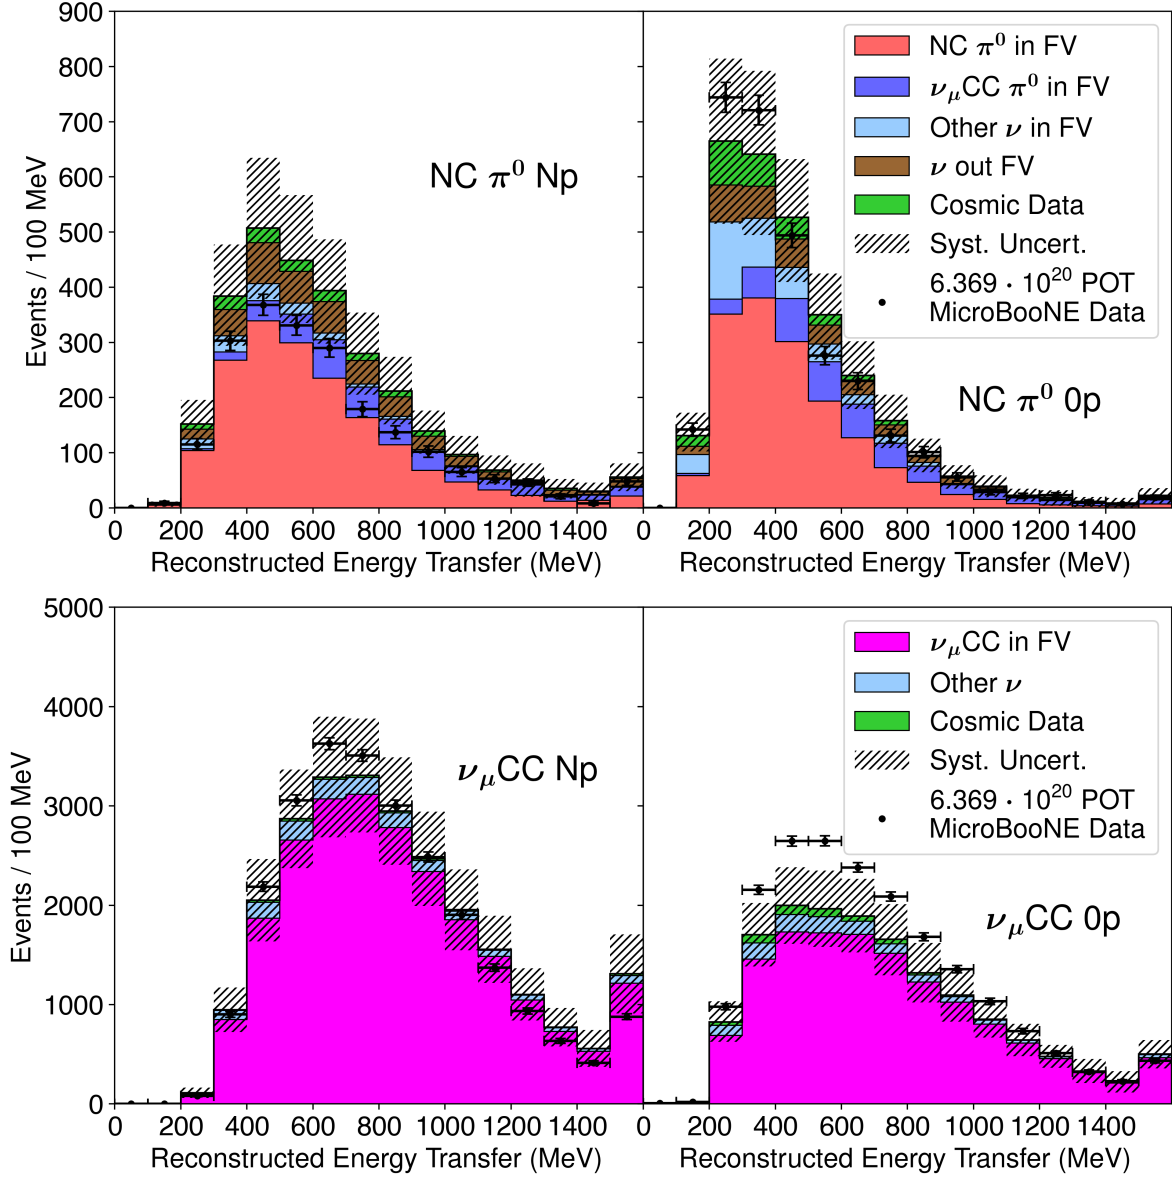

FIG. 6. NC  $\pi^0$  and  $\nu_\mu$ CC constraining channels. The rightmost bin in each subplot is an overflow bin.

## Appendix B: Sensitivities By Asimov Dataset

In Fig. 7 we show the sensitivities calculated using an Asimov dataset, a fake data set that exactly matches the prediction. The combination of Wire-Cell and Pandora is more sensitive than either reconstruction alone.

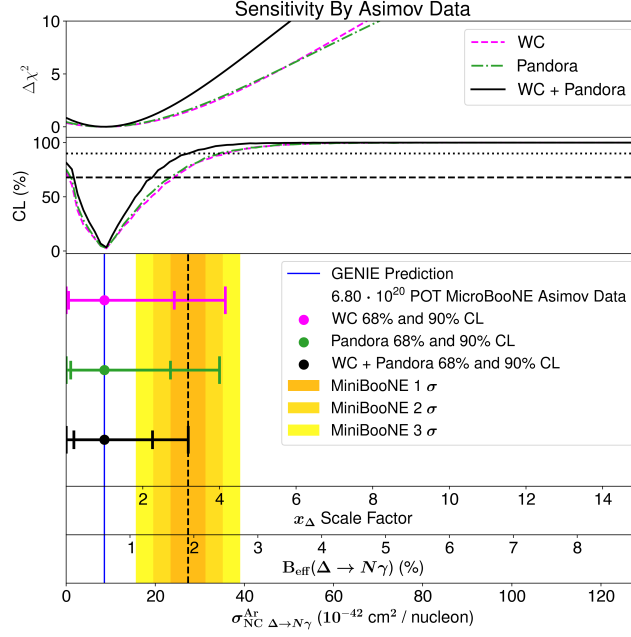

FIG. 7. NC  $\Delta \rightarrow N\gamma$  scaling exclusion sensitivities with Asimov data. The Pandora and Wire-Cell Asimov data samples correspond to  $6.80 \times 10^{20}$  and  $6.37 \times 10^{20}$  POT, respectively.

### Appendix C: Two Hypothesis Tests

In Fig. 8 we show the results of a two-hypothesis test. We generate 30,000 pseudo-experiments by sampling from our covariance matrix, including systematic and statistical uncertainties. We perform this both at the nominal NC  $\Delta \rightarrow N\gamma$  rate  $x_\Delta = 1$  as well as the alternative MiniBooNE LEE hypothesis NC  $\Delta \rightarrow N\gamma$  rate  $x_\Delta = 3.18$ . For each universe, we calculate  $\Delta\chi^2 = \chi_{x_\Delta=3.18}^2 - \chi_{x_\Delta=1}^2$ , and then compare distributions with data. We also compare with the median value to evaluate sensitivities.

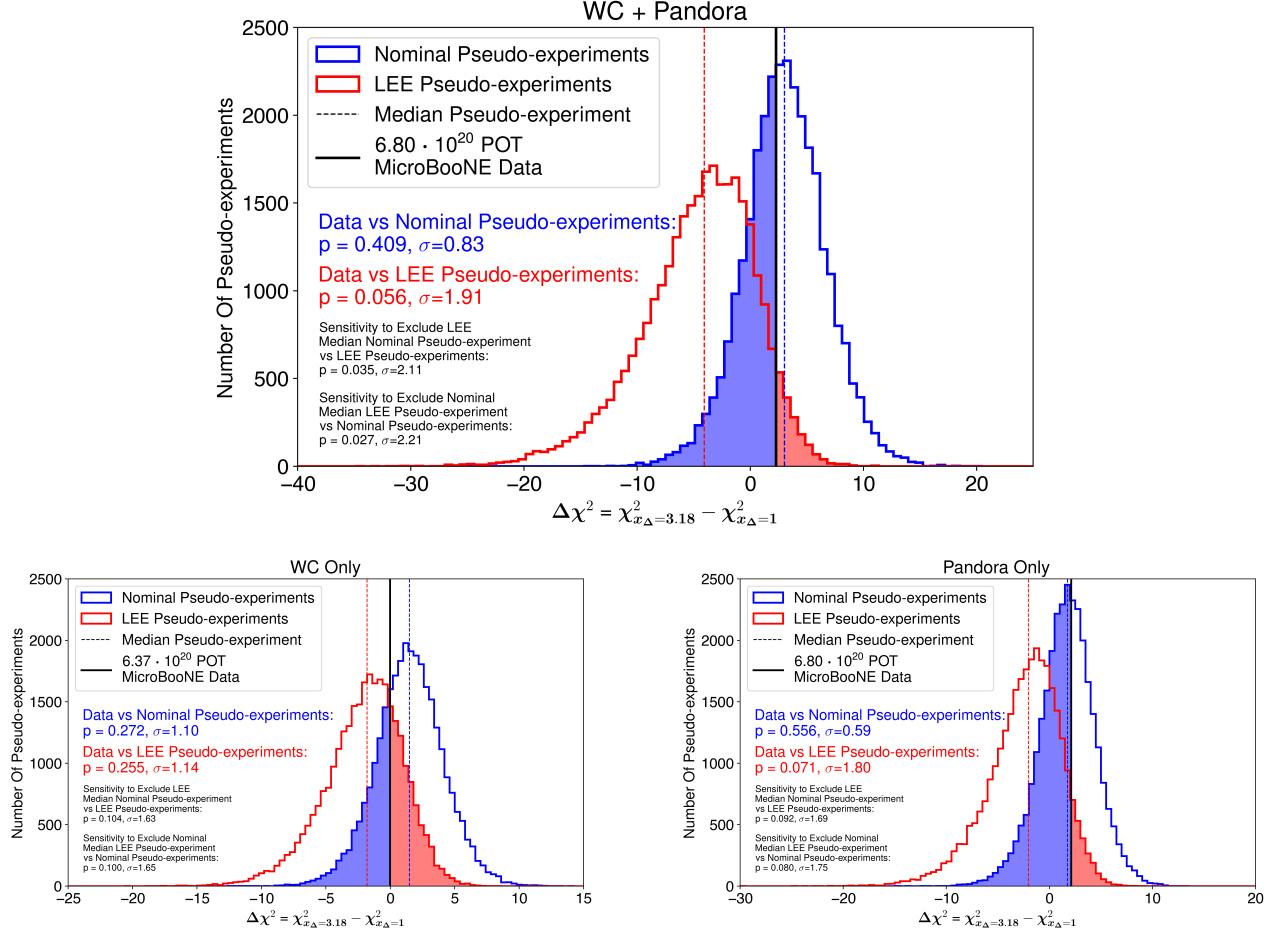

FIG. 8. Two hypothesis tests. For the top figure, the Pandora and Wire-Cell data samples correspond to  $6.80 \times 10^{20}$  and  $6.37 \times 10^{20}$  POT, respectively.

#### Appendix D: Efficiencies

Figure 9 shows NC  $\Delta \rightarrow N\gamma$  efficiencies for each selection as a function of true photon energy and angle. The angle  $\theta$  is measured with respect to the neutrino beam. There are some interesting differences between the selections. For example, for events with protons, Wire-Cell prefers forward events more strongly than Pandora. This represents one example of the type of difference that could cause the relatively low overlap between selected events.

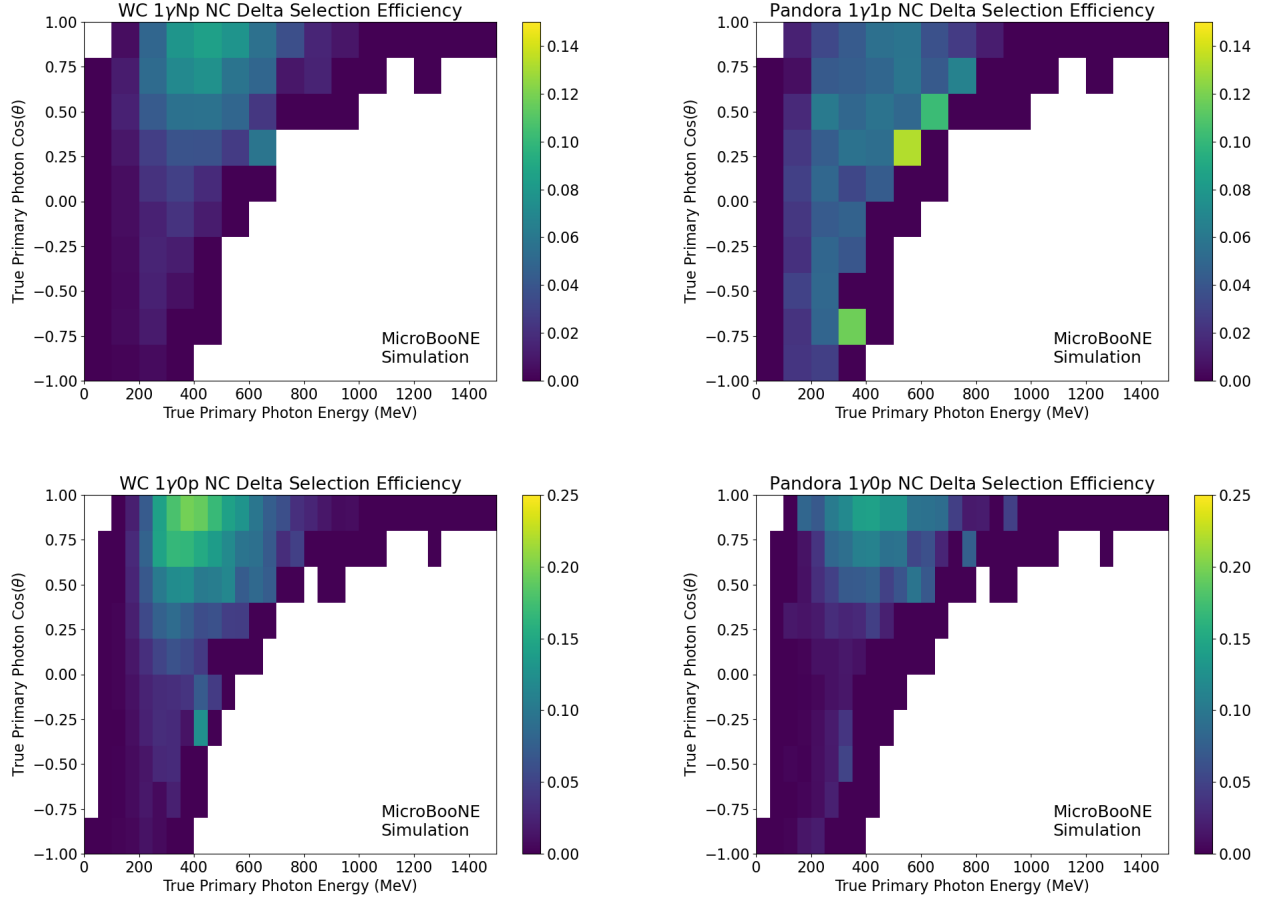

FIG. 9. NC  $\Delta \rightarrow N\gamma$  efficiencies for each selection as a function of true photon energy and angle.
